# Supplementary material for: MetroGNN: Metro Network Expansion with Reinforcement Learning
Source: arXiv:2403.09197 source file (2024-03-14)
Supplement: Supplementary file 1 [file appendix.tex]

\appendix
\section{Appendix}
\change{
\subsection{Rules for Metro Network Expansion}\label{app::constraints}}
The expansion of the metro network is subject to specific constraints to ensure the systematic and feasibility.
To fully describe these constraints, we introduce the following notations: $\mathcal{V}{\pm 1} \subset \mathcal{V}$ denotes the set of terminal stations for all metro lines, and $\mathcal{V}{\pm 2} \subset \mathcal{V}$ denotes the set of subterminal stations directly connected to the terminal stations in $\mathcal{V}_{\pm 1}$.
As introduced in Section \ref{app::mdp}, the expansion of metro network can be divided into the extension of existing lines and the construction of new lines. 
Regions available for the extension of existing lines must maintain reasonable station spacing and avoid sharp bends in the topology, as follows,
\begin{equation*}
    {t}^e(\mathcal{M}) = \{n_i\in\mathcal{N} \backslash \mathcal{V} \,|\, \text{EucDis}(n_i,n_j) \in [t3,t4]\wedge  \angle{n_i n_{j} n_{k}}\in [90^{\circ},180^{\circ}] \wedge n_j \in \mathcal{V}_{\pm 1}\wedge n_k\in \mathcal{V}_{\pm 2} \wedge (n_k,n_j)\in\mathcal{E}\}
\end{equation*}
where ${t}^e(\mathcal{M})$ represents the set of topologically feasible regions for extension, and $t_3$, $t_4$ are pre-defined thresholds.

Taking into account the budget constraint, we use $\mathcal{C}^e(n,\mathcal{M})$ to denote the minimum cost of adding region $n$ in an extended manner, then the set of the feasible regions for extension $\mathcal{X}^e(\mathcal{M},b_t)$ can be expressed as follows,
\begin{equation*}
    \mathcal{X}^e(\mathcal{M},b_t) = \{n\in {t}^e(\mathcal{M}) \,|\, |\mathcal{C}^e(n,\mathcal{M})| \leq b_t\}.
\end{equation*}

If a region is unsuitable for extension, we then consider whether it can serve as the starting station for a new metro line, topologically governed only by spacing rules,
\begin{equation*}
    {t}^c(\mathcal{M}) = \{n_i\in\mathcal{N}\backslash \mathcal{V}  \,|\, \text{EucDis}(n_i,n_j) \in [t3,t4]\}.
\end{equation*}

When considering limitations on the number of lines and budgets, the feasible regions for constructing new lines can be formulated as
\begin{equation*}
    \mathcal{X}^c(\mathcal{M},b_t,l_t) = \{n\in {t}^c(\mathcal{M}) \,|\, |\mathcal{C}^c(n,\mathcal{M})| \leq b_t \wedge l_t > 0\},
\end{equation*}
where $\mathcal{C}^c(n,\mathcal{M})$ denotes to the minimum cost of adding region $n$ in an constructive manner.

Despite the feasibility of regions, prioritization exists in the way regions expand the metro network.
Specifically, if region $n_i$ satisfies both $n_i\in \mathcal{X}^e(\mathcal{M},b_t)$ and $n_i \in \mathcal{X}^c(\mathcal{M},b_t,l_t)$ simultaneously, it will be prioritized as an extension of an existing line.
If $n_i$ can be used as an extension of multiple line, the least costly extension is considered.

\subsection{Preprocess of the Graph and OD Flows}\label{app::preprocess}
\noindent\textbf{Graph model.}
To facilitate proper metro network expansion, the delineation of regions follows specific preprocessing steps.
Initially, following the methodology outlined in \citet{wei2020city}, smaller regions that are geographically close to each other are merged.
This approach prevents excessive delineation of the road network structure.
Additionally, regions with larger areas but lower traffic demands, typically corresponding to remote areas such as mountains or rivers, are excluded. 
This step focuses the analysis to regions characterized by higher travel demand and activity.
Furthermore, regions that are distant from the initial metro lines are also omitted from consideration.
This is often due to budgetary constraints, as these remote regions are challenging to access within the constraints of the available budget.
Through these preprocessing steps, we can obtain a series of appropriate regions, laying the foundation for an efficient and fast strategy for metro network expansion.

\change{
\noindent\textbf{OD flows.}
We obtain inter-regional OD flows by processing a large number of user spatio-temporal trajectories. Specifically, if an individual travel from region A to region B and remains in B for at least 15 minutes, this travel event contributes a count of 1 to the OD flows from A to B. Furthermore, if the individual subsequently travels to region C, the entire movement will be considered as two separate trips: one from A to B and another from B to C.
}

\subsection{Implementation Details of Baseline}\label{app::baseline}
We compare our MetroGNN method with the following baselines.
\begin{itemize}[leftmargin=*]
    \item \textbf{GS} selects new region that meets the largest OD trips with previously selected region at each step.
    \item \textbf{GA} generates an initial population of metro lines and employs well-designed crossover and variance operators on individuals to generate the solutions.
    \change{We set the initial population size as 200 and limit the number of iteration to 2000.
    We also designed genetic operators for crossover and mutation which ensure the viability of the new population, and the probability of crossover and mutation are both 0.8.
    }
    \item \textbf{SA} commences with an initial solution and introduces stochastic modifications to explore the solution space.
    The algorithm progressively adapts to embrace the stochastic nature of suboptimal solutions during iterations, enabling it to transcend local optima and advance towards improved solutions.
    \change{We set the initial temperature to 1500, the cooling coefficient to 0.98, the termination temperature to 0.1, and 200 iterations for each temperature.
    Additionally, we set the acceptance threshold of SA to 0.1.}
    \item \textbf{ACO} runs with agents deposit pheromones on paths and establish connections with probabilistic rules.
    It iteratively updates pheromone levels based on evaluation metrics, thus steering the agents to better solutions.
    \change{We limit the maximum number of iterations of ACO to 3000 and include 128 instances per iteration.
    Other parameters of ACO aligns with ~\citet{yang2007parallel}.}
    \item \textbf{MP} formulates the metro expansion problem as an mixed integer programming model, and using solver to obtain solution.
    Considering the solution time, we use part of the expansion solutions of DRL-CNN and MetroGNN as a reference for the corridors to reduce to solution space.
    \change{Specifically, we consider regions within 10km of the existing metro network as the corridors, where regions are available candidates for metro network expansion.
    Additionally, the final metro network generated by MP may be discrete and need be manual adjustment.}
    \item \textbf{DRL-CNN} trains a actor-critic model to design new metro line based on the hidden state of current metro network. 
    At each step, it takes the embedded features as reference and the hidden state as query to select next region.
    \change{We adopt the network structure from ~\citet{wei2020city} to generate the metro network  expansion solutions.}
\end{itemize}

\subsection{Experiment Settings}\label{app::exp_setup}

For the metro network expansion task, there are four key parameters, construction cost, construction budget, initial metro lines (IL) and maximum new lines (ML).
We list all the values of above parameters for metro network expansion and the hyper-parameters of our method in Table \ref{tab::setting}, with default parameters indicated in bold.
Specifically, for the estimation of construction cost, we adopted the values of~\citet{wang2023designing} and fixed this setting in subsequent experiments.

\begin{table}[t]
\centering
\vspace{-5px}
\caption{Parameter values of MetroGNN.}
\label{tab::setting}
\vspace{-10px}
\begin{tabular}{ccc}
\toprule
\textbf{Category} & \textbf{Parameter} & \textbf{Value} \\
\midrule
\multirow{3}{*}{\bf{Cost}} 
& Cost per normal station ({million} RMB) & {300}\\
& Cost per interchange station ({million} RMB) & {600}\\
& Cost per kilometer ({million} RMB) & {500}\\
\hline
\multirow{3}{*}{\bf{Expansion}} & The number of Initial lines &  2,\textbf{4},6\\
& Maximum new lines  & 2,\textbf{3},4 \\
& Budget for expansion ({billion} RMB) & 40,\textbf{50},60\\
\hline
\multirow{5}{*}{\bf{Network}} & GNN layer & 2   \\
& GNN node dimension & 32 \\
& Attention Head & 2 \\
& Policy Head $\verb|MLP|_{p}$ & [32, 1] \\
& Value Head $\verb|MLP|_{v}$ & [32, 32, 1]  \\
\hline
\multirow{4}{*}{\bf{PPO}} & gamma & 0.99 \\
& tau & 0 \\
& Entropy Loss $\beta$ & 0.01  \\ 
& Value Loss $\gamma$ & 0.5  \\ 
\hline
\multirow{3}{*}{\bf{Train}} & optimizer & Adam \\
& weight decay & 0 \\
& learning rate & 0.0004 \\
\bottomrule
\end{tabular}
\end{table}

\change{
\subsection{The Transferability.}\label{app::transfer}}
In this section, we demonstrate how our proposed method adapts to the dynamics of growing cities and changing OD flows.
To simulate the expansion of the city, we initially remove the outer 20\% regions of Beijing and train MetroGNN on this reduced city for metro network expansion.
Subsequently, we apply the model to directly generate expansion solutions for the complete city area, and we also fine-tune the model for 10 additional iterations and evaluate its performance.
As shown in the Table \ref{tab:transfer}, the trained model can directly provide new metro network expansion solutions for the expanded city with performance close to that of DRL-CNN.
Remarkably, with further fine-tuning on the expanded city, the model produces outstanding expansion solutions, showcasing a significant improvement of more than 10.2\% compared to DRL-CNN.
Furthermore, recognizing that OD flows may change as urban functions shift, we explore the performance of the proposed method when confronted with varying OD trips.
As illustrated in Table \ref{tab:noise}, in the face of unpredictable OD trips, MetroGNN provides expansion solutions with an improvement of over 12.84\% compared to DRL-CNN, and the p-value $<$ 0.3\% further confirms the statistical significance of this substantial improvement.
Notably, the well-trained model can provide effective solutions for different urban areas within 20 seconds.
In contrast, other methods either yield solutions of poor quality or need to train from scratch for at least 3 hours, have difficulties in handling diverse urban scenarios.
These experiments on transferability highlight the excellent adaptability of our model in the face of changing urban regions and OD flows, underscoring its practical utility in real-world applications.

\begin{table}[t]
    \centering
    \vspace{-5px}
    \caption{The transferability of MetroGNN on expended city compared with DRL-CNN.
     Statistical significance is determined using a t-test to compare MetroGNN with DRL-CNN, denoted as $^*\text{p-value}<0.1$ and $^{**}\text{p-value}<0.05$.}
    \change{
        \begin{tabular}{c|c|c|c}
          \hline
          \textbf{From Scratch} & \textbf{Directly Transfer} & \textbf{Fine-Tune} & \textbf{DRL-CNN} \\
          \hline
          $18.93 \pm 0.87^{**}$ & $15.64 \pm 1.25$ & $17.39 \pm 1.04^{*}$ & $15.78 \pm 1.33$ \\
          \hline
        \end{tabular}
        }
    \label{tab:transfer}
\end{table}

\change{
\begin{table}[t]
    \centering
    \caption{The expansion performance with varying OD trips.Statistical significance is determined using a t-test to compare MetroGNN with DRL-CNN.}
    \change{
        \begin{tabular}{c*{10}{|c}}
          \hline
          \textbf{Method} & \textbf{1} & \textbf{2} & \textbf{3} & \textbf{4} & \textbf{5} & \textbf{6} & \textbf{7} & \textbf{8} & \textbf{9} & \textbf{10} \\
          \hline
          MPG & 12.71 & 12.49 & 11.87 & 9.18 & 13.54 & 15.77 & 14.53 & 18.80 & 13.61 & 14.86 \\
          \hline
          DRL-CNN & 15.93 & 14.31 & 15.86 & 15.10 & \textbf{16.76} & 15.71 & 16.57 & 17.29 & 16.57 & \textbf{17.98} \\
          \hline
          MetroGNN$^{**}$ & \textbf{18.63} & \textbf{16.93} & \textbf{17.91} & \textbf{16.58} & 16.69 & \textbf{19.44} & \textbf{18.83} & \textbf{20.17} & \textbf{17.79} & 17.48 \\
          \hline
          impr\% & 14.49 & 15.48 & 11.45 & 8.93 & -0.42 & 19.19 & 12.00 & 14.28 & 6.86 & -2.86 \\
          \hline
        \end{tabular}
        }
    \label{tab:noise}
    \vspace{-10px}
\end{table}
}

\begin{figure}[t]
    \centering
    \includegraphics[width=0.9\linewidth]{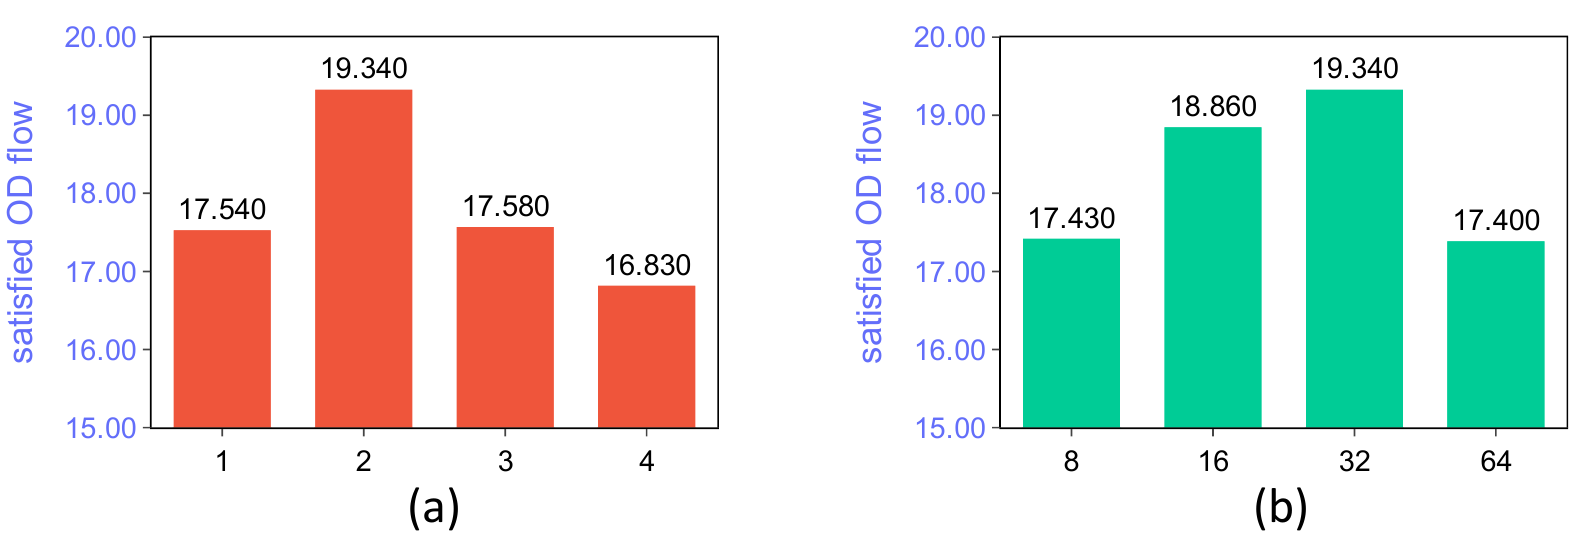}
    \vspace{-5px}
    \caption{
    Performance of MetroGNN with different values of (a) GNN layers (b) node dimension for the metro network expansion in Beijing, China.
    }
    \label{fig::hyper}
\end{figure}

\subsection{Hyper-parameter Study}\label{app::hyper}

We tune the hyper-parameters of MetroGNN with a series of hyper-parameter studys.
Specifically, we investigate two key hyper-parameters of our model in this section, which are the number of GNN layers, the dimenstion of GNN representations.

\noindent\textbf{GNN Layers.}
We propose a topology-aware and OD-aware message passing mechanism that propagates through heterogeneous edges in a single GNN layer.
Stacking multiple GNN layers can broaden each node's perception field, allowing it to aggregate features from distant nodes. 
However, excessive layer stacking can lead to oversmoothing and a decline in performance~\citep{chen2020measuring}.
We systematically vary the number of GNN layers and evaluate the variants' performance. 
Figure \ref{fig::hyper}(a) shows that the model with 2 GNN layers achieved optimal performance, while models with more or fewer layers exhibited varying degrees of performance degradation, with an average drop of 10\%.

\noindent\textbf{GNN Embedding Dimension.}
The dimension of GNN embeddings closely related to their representational capacity.
A higher dimension allows the model to capture more complex spatial relationships in OD flows between different regions.
However, excessively high dimensions can lead to overfitting, resulting in significant performance degradation.
Conversely, too low a dimension may inhibit the model's ability to learn effective representations.
Meanwhile, with too low dimension, model fails to learn effective representations.
We investigated the impact of varying the dimension of node embeddings on model performance. 
As illustrated in Figure \ref{fig::hyper}(b), setting the dimension to 32 for each node resulted in the best performance.
Increasing the dimension to 64 led to a performance decrease of over 10\%, while reducing it to 16 and 8 resulted in performance degradations of 2.5\% and 9.8\%, respectively.
\change{
\subsection{Metro Network Expansion with Equity} \label{app::equity}}
\begin{table}[t]
    \centering
    \caption{Expansion with reward weights $\alpha=1.0,\beta=0.0$}
    \change{
        \vspace{-5px}
        \begin{tabular}{|l|c|c|c|}
          \hline
          \textbf{Method} & \textbf{OD} & \textbf{equity} & \textbf{weighted} \\
          \hline
          DRL-CNN & $15.78\pm1.33$ & $12.32\pm1.46$ & $15.78\pm1.33$ \\
          MetroGNN & $18.93\pm0.87^{**}$ & $11.58\pm0.26$ & $18.93\pm0.87^{**}$ \\
          \hline
          impr\% v.s. DRL-CNN & 19.96 & -6.01 & 19.96 \\
          \hline
        \end{tabular}
        \vspace{-5px}
        }
    \label{tab:w1}
\end{table}

\begin{table}[t]
    \centering
    \caption{Expansion with reward weights $\alpha=0.5,\beta=0.5$}
    \change{
    \vspace{-5px}
        \begin{tabular}{|l|c|c|c|}
          \hline
          \textbf{Method} & \textbf{OD} & \textbf{equity} & \textbf{weighted} \\
          \hline
          DRL-CNN & $13.20\pm1.72$ & $20.72\pm1.94$ & $16.96\pm1.80$ \\
          MetroGNN & $16.50\pm1.14^{**}$ & $23.90\pm1.28^{*}$ & $20.20\pm1.21^{**}$ \\
          \hline
          impr\% v.s. DRL-CNN & 25.00 & 15.35 & 19.10 \\
          \hline
        \end{tabular}
        \vspace{-10px}
        }
    \label{tab:w2}
\end{table}

\begin{table}[t]
    \centering
    \caption{Expansion with reward weights $\alpha=0.0,\beta=1.0$}
    \change{
    \vspace{-5px}
        \begin{tabular}{|l|c|c|c|}
          \hline
          \textbf{Method} & \textbf{OD} & \textbf{equity} & \textbf{weighted} \\
          \hline
          DRL-CNN & $11.86\pm2.32$ & $26.70\pm2.16$ & $26.70\pm2.16$ \\
          MetroGNN & $10.49\pm1.85$ & $28.42\pm1.49^{*}$ & $28.42\pm1.49^{*}$ \\
          \hline
          impr\% v.s. DRL-CNN & -11.55 & 6.44 & 6.44 \\
          \hline
        \end{tabular}
        \vspace{-10px}
        }
    \label{tab:w3}
\end{table}

While the construction of metro networks is primarily driven by public transportation demands, social factors like equity also play a crucial role in shaping their layout~\citep{arsenio2016sustainable,behbahani2019conceptual}.
We first define the inequity of a metro network as the variance in the distance from all regions to the metro network.
Let $\text{EucDis}(n_i,\mathcal{M})$ denotes to the shortest Euler distance from region $n_i$ to the metro network $\mathcal{M}$, then the inequity of $\mathcal{M}$ can be formulated as follows,
\begin{equation}
    \text{IE}(\mathcal{M}) = \dfrac{1}{|\mathcal{N}|}\sum_{n_i\in\mathcal{N}}(\text{EucDis}(n_i,\mathcal{M}) - \dfrac{1}{|\mathcal{N}|}\sum_{n_j\in\mathcal{N}}\text{EucDis}(n_j,\mathcal{M}))^2,
\end{equation}
and the equity improvement of the expansion is defined as the decrease in inequity $\text{IE}(\mathcal{M}_T) - \text{IE}(\mathcal{M}_0)$, where $\mathcal{M}_T$ represents the expanded metro network and $\mathcal{M}_0$ represents the original metro network.
When equity is included as an evaluation metric, the metro network expansion transforms into a multi-objective optimization problem.
The rewards of the MDP can be expressed as a weighted sum of two metrics as follows,
\begin{equation}
    R_t = \alpha * ({C_{od}(\mathcal{M}_t)-C_{od}(\mathcal{M}_{t-1})}) + \beta * (\text{IE}(\mathcal{M}_t) - \text{IE}(\mathcal{M}_{t-1})), \label{eq:equ}
\end{equation}
where $\alpha$ and $\beta$ are the weights of the OD flows and equity, respectively.
By varying the weighting factors in the rewards, we can generate expansion solutions with different preferences.
As presented in Tables \ref{tab:w1} and \ref{tab:w3}, when considering only the satisfaction of OD flows or equity individually, our method provides significantly superior expansion schemes compared to DRL-CNN, with improvements of 19.96\% and 6.44\%, respectively. 
Notably, when factoring in both travel demands and equity, MetroGNN outperforms DRL-CNN on both metrics, showcasing an average improvement of more than 20.1\%.
The powerful graph characterization capability of the GNN module enables the learning of intricate OD flow characteristics, while the attentive policy network correlates each region with the metro network layout, facilitating the generation of fairer expansion solutions.
